# Supplementary material for: Mitigating Open-Vocabulary Caption Hallucinations
Source: arXiv:2312.03631 source file (2024-10-16)
Supplement: Supplementary file 1 [file supp.tex]

\documentclass[10pt,twocolumn,letterpaper]{article}

\usepackage[review]{cvpr}      %

\usepackage{graphicx}
\usepackage{amsmath}
\usepackage{amssymb}
\usepackage{booktabs}
\usepackage[dvipsnames]{xcolor}
\usepackage{tabularx}
\usepackage{multirow}
\usepackage{pifont}
\usepackage{subcaption}
\usepackage{caption}
\usepackage[normalem]{ulem}
\usepackage{fixltx2e}
\usepackage{soul}
\usepackage[export]{adjustbox}
\usepackage{colortbl}
\usepackage{makecell}
\usepackage{array}
\usepackage{ragged2e}

\definecolor{cvprblue}{rgb}{0.21,0.49,0.74}
\usepackage[pagebackref,breaklinks,colorlinks,citecolor=cvprblue]{hyperref}

\input{macros}

\usepackage[capitalize]{cleveref}
\crefname{section}{Sec.}{Secs.}
\Crefname{section}{Section}{Sections}
\Crefname{table}{Table}{Tables}
\crefname{table}{Tab.}{Tabs.}

\title{\methodname{}: Multi-Objective Reinforcement Mitigating Caption Hallucinations \\ -- Supplementary Material --}

\author{First Author\\
Institution1\\
Institution1 address\\
{\tt\small firstauthor@i1.org}
\and
Second Author\\
Institution2\\
First line of institution2 address\\
{\tt\small secondauthor@i2.org}
}

\begin{document}

\maketitle

\thispagestyle{empty} %
\setcounter{tocdepth}{2}

\tableofcontents
\bigskip

\input{supp_00_viz}
\input{supp_01_details}
\input{supp_02_comparisons}
\input{supp_03_extended_rw}

{\small
\bibliographystyle{ieee_fullname}
\bibliography{egbib}
}

\end{document}
